# Supplementary material for: Numerical Simulation of Superparamagnetic Nanoparticle Motion in Blood Vessels for Magnetic Drug Delivery
Source: arXiv:2110.01988 source file (2021-10-07)
Supplement: Supplementary file 1 [file appendix1.tex]

\section{Appendix} \label{sec:appendix}
